# Supplementary material for: On Universality of Non-Separable Approximate Message Passing Algorithms
Source: arXiv:2506.23010 source file (2026-09-11)
Supplement: Supplementary file 1 [file SupplementCommands.tex]

\RequirePackage{mathrsfs}

\theoremstyle{plain}

\numberwithin{theorem}{section}
\numberwithin{equation}{section}

\renewcommand{\thesubfigure}{\Alph{subfigure}}

\def\PP{\mathbb{P}}
\def\EE{\mathbb{E}}
\def\RR{\mathbb{R}}
\def\NN{\mathbb{N}}
\def\bA{\mathbf{A}}
\def\bB{\mathbf{B}}
\def\bD{\mathbf{D}}
\def\bE{\mathbf{E}}
\def\bG{\mathbf{G}}
\def\bK{\mathbf{K}}
\def\bM{\mathbf{M}}
\def\bP{\mathbf{P}}
\def\bO{\mathbf{O}}
\def\bS{\mathbf{S}}
\def\bT{\mathbf{T}}
\def\bU{\mathbf{U}}
\def\bW{\mathbf{W}}
\def\bX{\mathbf{X}}
\def\bY{\mathbf{Y}}
\def\bZ{\mathbf{Z}}
\def\bb{\mathbf{b}}
\def\be{\mathbf{e}}
\def\bi{\mathbf{i}}
\def\bj{\mathbf{j}}
\def\bk{\mathbf{k}}
\def\br{\mathbf{r}}
\def\bu{\mathbf{u}}
\def\bv{\mathbf{v}}
\def\bw{\mathbf{w}}
\def\bx{\mathbf{x}}
\def\by{\mathbf{y}}
\def\bz{\mathbf{z}}
\def\bgamma{\boldsymbol{\gamma}}
\def\btheta{\boldsymbol{\theta}}
\def\bxi{\boldsymbol{\xi}}
\def\bOmega{\boldsymbol{\Omega}}
\def\bSigma{\boldsymbol{\Sigma}}
\def\bTheta{\boldsymbol{\Theta}}
\def\bone{\mathbf{1}}
\def\cA{\mathcal{A}}
\def\cB{\mathcal{B}}
\def\cC{\mathcal{C}}
\def\cD{\mathcal{D}}
\def\cE{\mathcal{E}}
\def\cF{\mathcal{F}}
\def\cG{\mathcal{G}}
\def\cI{\mathcal{I}}
\def\cK{\mathcal{K}}
\def\cL{\mathcal{L}}
\def\cN{\mathcal{N}}
\def\cP{\mathcal{P}}
\def\cQ{\mathcal{Q}}
\def\cS{\mathcal{S}}
\def\cT{\mathcal{T}}
\def\cV{\mathcal{V}}
\def\sP{\mathscr{P}}

\def\mat{\operatorname{mat}}
\def\vec{\operatorname{vec}}
\def\Id{{\operatorname{Id}}}
\def\diag{\operatorname{diag}}
\def\Tr{\operatorname{Tr}}
\def\sign{\operatorname{sign}}
\def\div{\operatorname{div}}
\def\Var{\operatorname{Var}}
\def\Fro{\mathrm{F}}
\def\op{\mathrm{op}}
\def\val{\mathrm{val}}
\def\vecval{\mathrm{vec\text{-}val}}
\def\GOE{\mathrm{GOE}}
\def\<{\langle}
\def\>{\rangle}
\def\1{1 \!\! 1}
\def\Oprec{O_{\prec}}
\def\Wg{\operatorname{Wg}}
\def\sym{\mathrm{sym}}
\def\alt{\mathrm{alt}}
\def\c{\mathbf{c}}
\renewcommand{\ss}[1]{[#1]}

\makeatletter
\newcommand*{\rom}[1]{\expandafter\@slowromancap\romannumeral #1@}
\makeatother

\renewcommand{\u}{\underline}
